# Supplementary material for: EgoPrompt: Prompt Learning for Egocentric Action Recognition
Source: arXiv:2508.03266 source file (2025-08-07)
Supplement: Supplementary file 1 [file appendix.tex]

\section{Supplementary Material}
This supplementary document provides additional technical details, ablations, and empirical studies to further support the contributions of the main paper. Specifically, we present:
\begin{enumerate}
    \item A detailed mathematical formulation of the multi-layer prompt mapping mechanism used in MaPLe.
    \item Architectural overview of the \textbf{LaVILA} backbone used in EgoPrompt, including its temporal-spatial attention design, contrastive pretraining, and adaptation within our prompt learning framework.
    \item Empirical analysis of component-specific template design and its impact on performance. 
    \item An ablation study on the use of deep prompting strategies, examining how hierarchical prompt insertion affects generalization under both within- and cross-dataset evaluation settings.
    \item A comprehensive overview of training and backbone hyperparameter choices, along with sensitivity studies to assess their robustness.
    \item Comparison of training and inference efficiency across different methods and configurations.
    \item More results on the size of the Unified Prompt Pool, examining how varying the number of prompt pairs affects generalization performance across domains.

\end{enumerate}
These supplementary materials aim to provide deeper insights into the design choices and practical implications of our proposed \textbf{EgoPrompt} framework.

\subsection{Hierarchical Prompt Mapping in MaPLe}
MaPLe~\cite{khattak2023maple} introduces a multi-layer hierarchical prompt learning strategy to bridge vision and language modalities via deep prompt interaction. This approach enables effective semantic alignment across transformer layers. We formally describe the key components and derivation below.

\noindent\textbf{Prompt Propagation in the Text Encoder}
Let the text encoder $\mathcal{T} = \{\mathcal{T}_k\}_{k=1}^K$ be a $K$-layer Transformer. At each layer $k$, MaPLe introduces learnable textual prompts $\bm{p}_t^k \in \mathbb{R}^{L_t \times d}$, where $L_t$ is the prompt length and $d$ is the embedding dimension.

At each layer, the prompt is concatenated with the intermediate feature $\hat{e}_{k-1}$ from the previous layer and passed through the $k$-th Transformer layer:
\begin{equation}
\hat{e}_k = \mathcal{T}_k\left([\hat{e}_{k-1}; \bm{p}_t^{k-1}]\right), \quad k = 1, \dots, K,
\label{text_prompt}
\end{equation}
where $[\cdot ; \cdot]$ denotes concatenation along the token sequence dimension. The final output $\hat{e}_K$ is used to derive the class-level text embedding:
\begin{equation}
w_i = \text{CLS}(\hat{e}_K^{(i)}), \quad i = 1, \dots, N,
\label{text_cls}
\end{equation}
where $\hat{e}_K^{(i)}$ is the processed prompt of the $i$-th class and $\text{CLS}(\cdot)$ denotes the extraction of the class token embedding.

\noindent\textbf{Prompt Mapping to the Video Modality}
To enable modality alignment, MaPLe projects the text-aware prompts $\bm{p}_t^k$ into the video modality through a linear mapping:
\begin{equation}
\bm{p}_v^k = \mathcal{M}_k(\bm{p}_t^k), \quad k = 1, \dots, K,
\label{maple_projection}
\end{equation}
where $\mathcal{M}_k: \mathbb{R}^{L_t \times d} \rightarrow \mathbb{R}^{L_v \times d}$ is a learnable linear transformation for layer $k$, producing video-aware prompts $\bm{p}_v^k$.

\begin{figure}[t]
  \centering
  \includegraphics[width=1\linewidth]{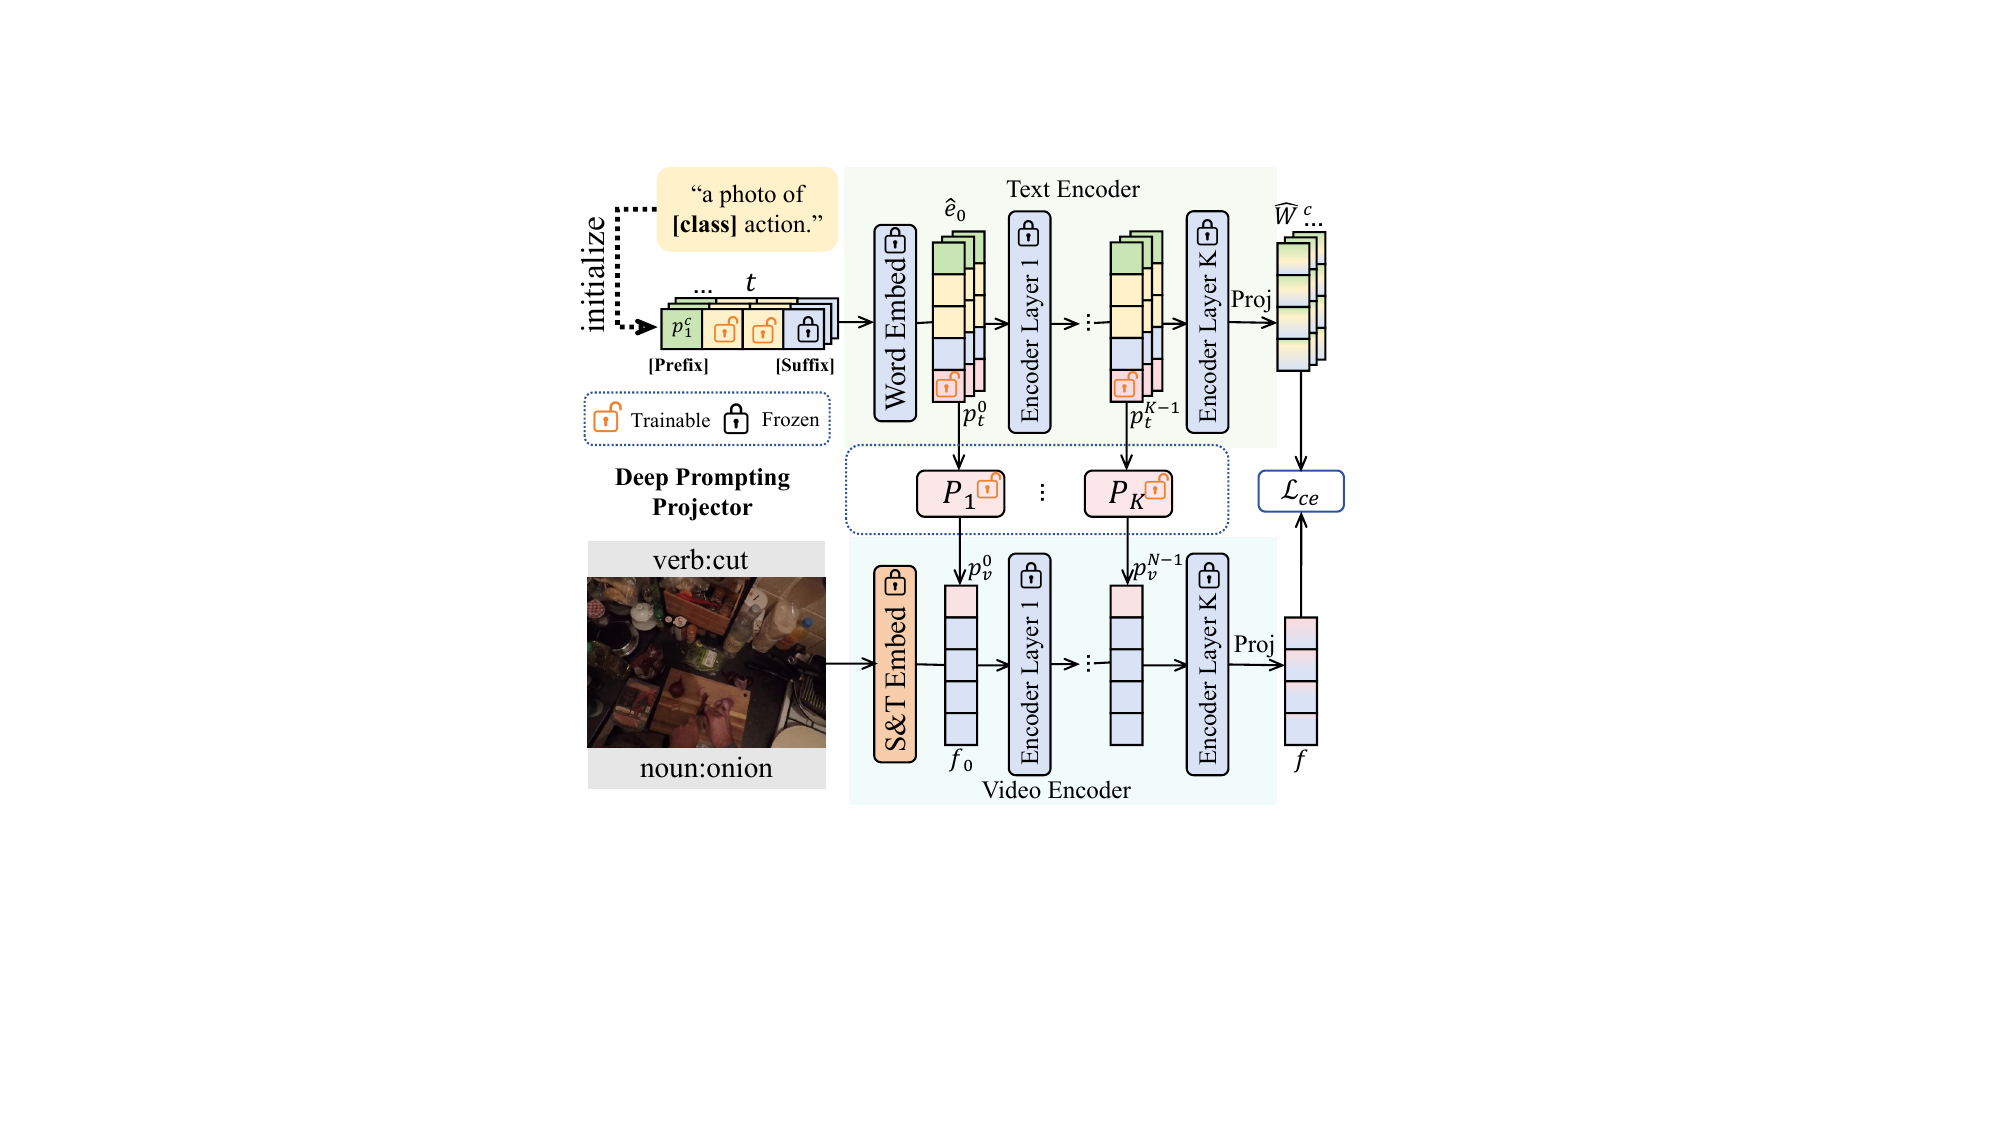}
  \caption{Overall framework of MaPLe. }
  \label{framework}
  \vspace{-0.8em}
\end{figure}

\noindent\textbf{Prompt Injection in the Video Encoder}
Let the video encoder be $\mathcal{V} = \{\mathcal{V}_k\}_{k=1}^K$, operating on the visual representation $f_0$ (e.g., video patch embeddings). At each layer $k$, the mapped video prompts $\bm{p}_v^{k-1}$ are concatenated with the intermediate representation $f_{k-1}$ and passed into the next layer:
\begin{equation}
f_k = \mathcal{V}_k\left([f_{k-1}; \bm{p}_v^{k-1}]\right), \quad k = 1, \dots, K.
\label{video_prompt}
\end{equation}
This progressive injection allows the visual encoder to incorporate semantically aligned prompt information across layers, facilitating deeper vision-language interaction.

\noindent\textbf{Final Representation and Classification}
After $K$ layers, the final feature $f_K$ is used to compute the similarity with class embeddings $w_i$ from Eq.~\eqref{text_cls}. The classification probability is calculated using a temperature-scaled cosine similarity:
\begin{equation}
\text{sim}(x, i) = \frac{\cos(f_K(x), w_i)}{\tau}, \quad i = 1, \dots, N,
\end{equation}
where $\tau$ is a temperature parameter. The model is optimized via cross-entropy loss:
\begin{equation}
\mathcal{L}_{\text{ce}} = - \log \frac{\exp(\text{sim}(x, y))}{\sum_{i=1}^N \exp(\text{sim}(x, i))}.
\end{equation}

\begin{table*}
\caption{\textbf{Impact of Template Design on Generalization Performance.} Results are reported on the ``From E4D to EK'' setting.} 
\label{templates}
\centering
\small
\begin{tabular}{@{}l|ccc|ccc@{}}
\hline
 \multirow{2}{*}{Templates}           & \multicolumn{3}{c|}{Nouns}                  & \multicolumn{3}{c}{Verbs}                 \\

           & \multicolumn{1}{c}{E4D}                     & \multicolumn{1}{c}{EK}                        &
             \multicolumn{1}{c|}{hm}                      & \multicolumn{1}{c}{E4D}                         & 
             \multicolumn{1}{c}{EK}                       & \multicolumn{1}{c}{hm}                         \\
\hline
a photo of [class]               &  \textbf{43.87}& 33.51 & 38.00                       & 28.14 & 45.32 & 34.72                           \\
a photo of a [class] action      &  42.07 & 31.86  & 36.26                        & \textbf{29.65} & \textbf{47.81} & \textbf{36.60}               \\ 
a photo of actioning on [class]  &  43.26 & \textbf{34.81} & \textbf{38.58}                        & 28.40 & 46.53 & 35.27                         \\
\hline
\end{tabular}
\end{table*}

\begin{table*}[t]
\caption{\textbf{Training time and parameters comparison.} Training efficiency of EgoPrompt compared with existing baselines. "Params" reports trainable parameters in millions and relative to full LaVILA. "Training time" is measured in seconds per batch on a single A100 GPU.}
\label{complexity}
\centering
\small
\begin{tabular}{l|ccccc}
\hline
\textbf{Methods} & \textbf{Params } & \textbf{ LaVILA} & \textbf{Training Time} & \multicolumn{2}{c}{\textbf{From E4D to EK}}\\
& (M) & (\%) & (s/bs) & Verb(\%) & Noun(\%) \\
\hline
X-MIC & 12.37 & 1.32\% & 3.51 & 28.3 & 39.5\\
MaPLe & 16.80 & 1.79\% & 3.79 & 32.8 & 44.4\\
SFT (Full Fine-tuning) & 938.0 & 100\% & 6.25 & 21.7 & 16.8 \\
\rowcolor{blue!10}
EgoPrompt & 18.07 & 1.92\% & 3.82 & 35.8 & 47.9 \\
\hline
\end{tabular}
\end{table*}

\begin{table*}[t]
\caption{\textbf{Effect of Deep Prompting Strategy.} Results are reported on the ``From E4D to EK'' generalization setting.}
\label{deep_prompting}
\centering
\small
\begin{tabular}{@{}l|ccc|ccc@{}}
\hline
\multirow{2}{*}{\textbf{Setting}} & \multicolumn{3}{c|}{Nouns (\%)} & \multicolumn{3}{c}{Verbs (\%)} \\
\cline{2-7}
 & E4D & EK & hm & E4D & EK & hm \\
\hline
w/o Deep Prompting & 41.10 & 28.65 & 33.72 & 27.46 & 44.96 & 34.00 \\
\rowcolor{blue!10}
w/ Deep Prompting & \textbf{42.93} & \textbf{35.75} & \textbf{39.01} & \textbf{29.71} & \textbf{47.89} & \textbf{36.67} \\
\hline
\end{tabular}
\end{table*}

\subsection{Details of LaVILA Backbone}
To provide further clarity on the model architecture, we present a detailed overview of the LAVILA~\cite{lavila} backbone adopted in EgoPrompt.

\noindent\textbf{Video Encoder.}  
LAVILA employs a TimesFormer-based~\cite{bertasius2021timesformer} video encoder, where each transformer block is composed of three components: a temporal attention layer, a spatial attention layer, and a multi-layer perceptron (MLP), each followed by residual connections. Specifically:
\begin{equation}
    z_{k-1} = \text{TimeAttn}(e_{k-1}) + e_{k-1},
\end{equation}
\begin{equation}
    z'_{k-1} = \text{SpaceAttn}(z_{k-1}) + z_{k-1},
\end{equation}
\begin{equation}
    e_k = \text{MLP}(z'_{k-1}) + z'_{k-1},
\end{equation}
where $e_k$ denotes the output embedding of the $k$-th transformer block, and $z_{k-1}$, $z'_{k-1}$ are intermediate representations.  
The spatial attention operates within individual frames, while the temporal attention captures dependencies across frames at corresponding spatial locations.

\noindent\textbf{Text Encoder.}  
For textual input, LAVILA employs GPT-2 XL~\cite{lagler2013gpt2} to generate rich supervision from large-scale language models. However, in EgoPrompt, we replace it with the CLIP text encoder to enable more effective contrastive learning with visual features.

\noindent\textbf{Cross-modal Fusion.}  
To align video and text modalities, LAVILA introduces a cross-attention module consisting of a cross-attention layer followed by a feed-forward network (FFN). Layer normalization is applied before both components to stabilize training:
\begin{itemize}
    \item Cross-Attn $\rightarrow$ Add \& Norm $\rightarrow$ FFN $\rightarrow$ Add \& Norm
\end{itemize}

\noindent\textbf{Backbone Variants.}  
We adopt two variants of the TimesFormer-based video encoder:
\begin{itemize}
    \item \textbf{TSF-B:} 12 transformer blocks (ViT-B/16).
    \item \textbf{TSF-L:} 24 transformer blocks (ViT-L/16).
\end{itemize}
These variants allow us to evaluate the scalability and adaptability of EgoPrompt under different model capacities.

\noindent\textbf{Usage in EgoPrompt.}  
During downstream training, the video encoder from the pre-trained LAVILA is directly reused in EgoPrompt. All video representations are extracted using this encoder, while the prompt learning modules (e.g., prompt pool, fusion layers) are trained to adapt the representations for egocentric action recognition.

\subsection{Empirical Analysis of Template Design}
In EgoPrompt, hand-crafted textual templates are not merely used as initialization for prompt learning—as done in prior methods like CoOp—but also serve as semantic priors to guide the optimization of soft prompts through the knowledge-guided loss $\mathcal{L}_{kg}$. This design encourages the learned prompts to preserve class-level generalization from human-designed descriptions.

To explore the impact of different template designs under this constraint, we evaluate several candidate prompts for both noun and verb components. As summarized in Table~\ref{templates}, the following observations emerge:
For \textbf{nouns}, the template \textit{a photo of actioning on [class]''} yields the best harmonic mean accuracy (38.58\%), as it captures the object’s role within an interactive context—better aligning with the HOI nature of egocentric understanding. 
For \textbf{verbs}, the template \textit{a photo of a [class] action''} outperforms the others (36.60\%), as it directly emphasizes the action itself and provides clearer cues for temporal behavior recognition. 

Based on these results, we adopt a photo of a [class] action'' as the default verb prompt and a photo of actioning on [class]'' for nouns in all subsequent experiments. These choices ensure that the knowledge-guided loss effectively regularizes the prompt learning process with component-aware textual priors.

\begin{figure}
    \centering
    \includegraphics[width=0.8\linewidth]{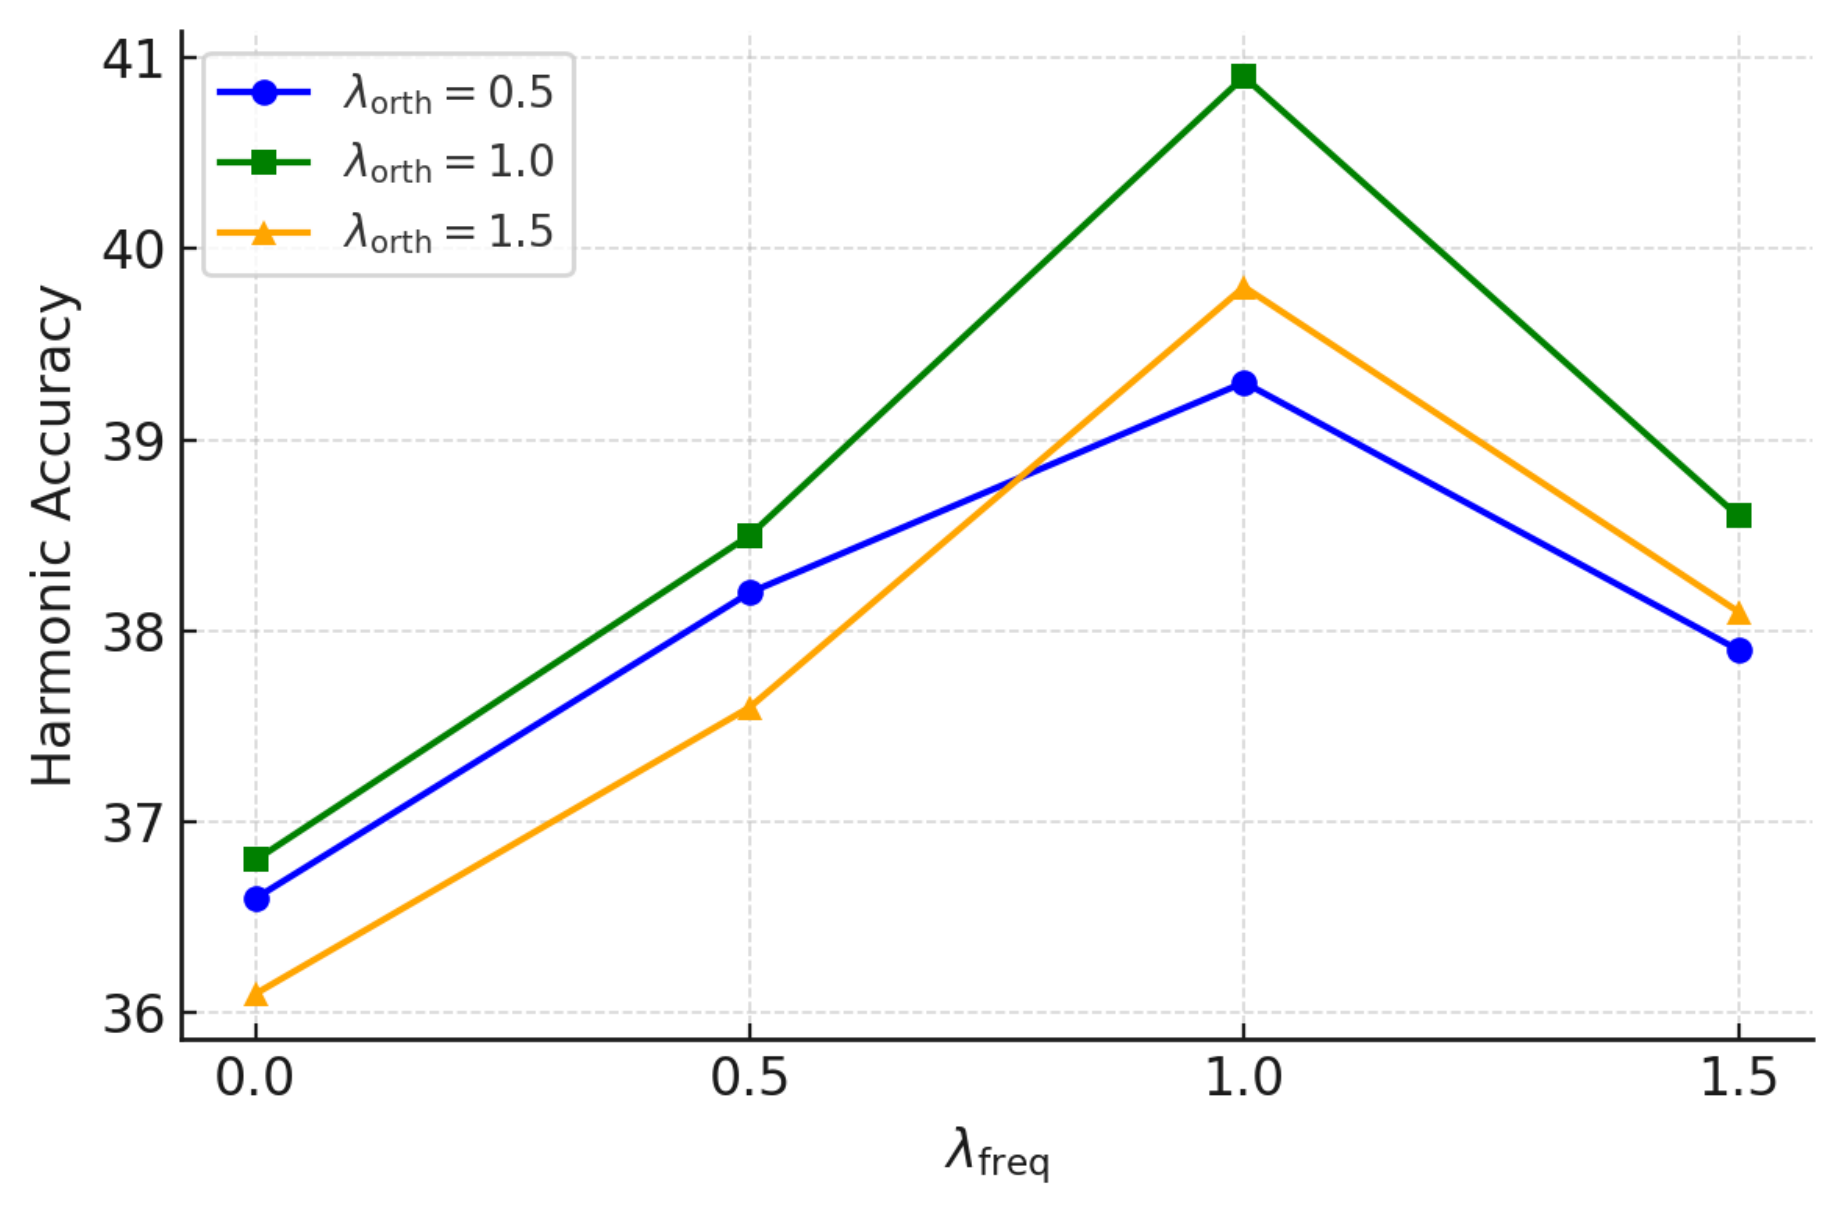}
    \caption{\textbf{Effect of $\lambda_{\text{freq}}$ under different $\lambda_{\text{orth}}$ settings.}}
    \label{freq}
    \vspace{-1.0em}
\end{figure}

\begin{figure}
    \centering
    \includegraphics[width=0.8\linewidth]{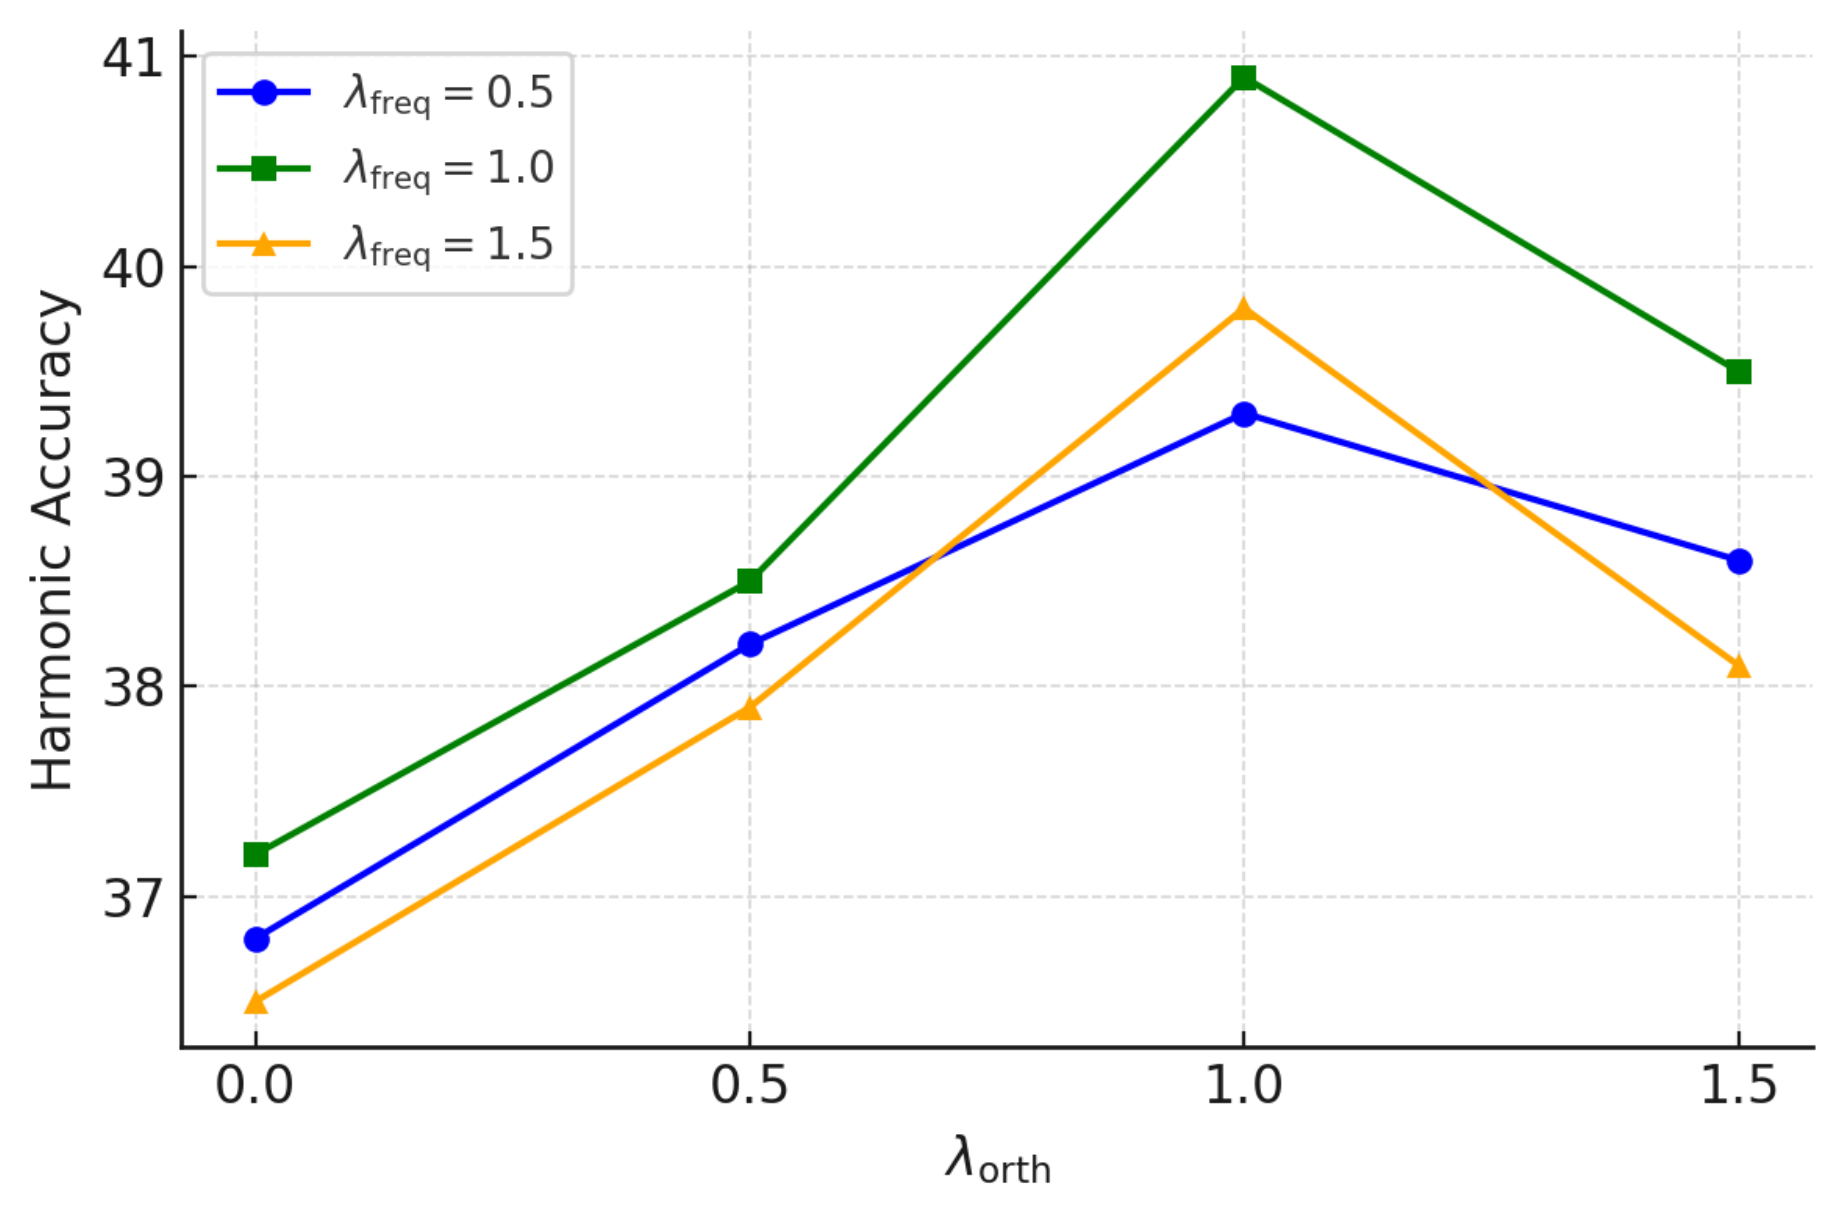}
    \caption{\textbf{Effect of $\lambda_{\text{orth}}$ under different $\lambda_{\text{freq}}$ settings.}}
    \label{orth}
    \vspace{-1.0em}
\end{figure}

\subsection{Effect of Deep Prompting Strategy}
To evaluate the contribution of deep prompting in EgoPrompt, we conduct an ablation study comparing performance with and without the deep prompting mechanism under the ``From E4D to EK'' cross-dataset generalization setting. As shown in Table~\ref{deep_prompting}, incorporating deep prompting leads to consistent improvements across both nouns and verbs.
Specifically, deep prompting improves noun accuracy on the target domain (EK) from 28.65\% to 35.75\%, and verb accuracy from 44.96\% to 47.89\%. This results in harmonic mean (hm) gains of +5.29\% for nouns and +2.67\% for verbs. These improvements demonstrate that deep prompting enables more expressive and task-adaptive representations by progressively injecting prompt information across transformer layers rather than relying solely on shallow prompt initialization.
The results validate that deep prompting serves as a powerful mechanism to enhance the semantic capacity of EgoPrompt, leading to better transferability and more robust performance under domain shifts.

\subsection{Training and Inference Efficiency}
Table~\ref{complexity} compares the training efficiency and cross-dataset generalization performance of EgoPrompt against several baselines. Despite introducing an additional interaction mechanism via the Unified Prompt Pool, EgoPrompt remains lightweight with only 1.92\% of LaVILA’s trainable parameters and a per-batch training time of 3.82 seconds—comparable to adapter-based methods such as MaPLe (1.79\%, 3.79s) and significantly lower than full fine-tuning (SFT), which consumes 100\% parameters and 6.25s/bs.

In terms of generalization from Ego4D to Epic-Kitchens, EgoPrompt achieves the highest accuracy on both verbs (35.8\%) and nouns (47.9\%), outperforming all baselines by notable margins. While SFT has access to full model capacity, it suffers from overfitting and fails to generalize well (21.7\% verb, 16.8\% noun). These results demonstrate that EgoPrompt not only improves cross-domain robustness but also achieves strong generalization with minimal training overhead, offering an efficient and scalable alternative for egocentric video understanding.

\begin{table}[t]
\caption{\textbf{Training and Model Configuration Parameters.}}
\label{tab:hyperparams}
\centering
\begin{tabular}{@{}c|c@{}}
\hline
\textbf{Category} & \textbf{Setting} \\
\hline
\multicolumn{2}{c}{\textit{Optimizer (AdamW)}} \\
\hline
Learning Rate (LR) & 0.0001 \\
Adam $\beta_1$ & 0.9 \\
Adam $\beta_2$ & 0.98 \\
Weight Decay & 0.01 \\
Warm-up Epochs & 2 \\
Warm-up Strategy & Linear \\
Minimum LR during Warm-up & 2e-5 \\
\hline
\multicolumn{2}{c}{\textit{Video Input (LaVILA)}} \\
\hline
Number of Key Frames & 16 \\
\hline
\multicolumn{2}{c}{\textit{Prompt Mapping (MaPLe)}} \\
\hline
MLP Layers in MaPLe & 2 \\
MLP Hidden Dimension & 512 \\
\hline
\end{tabular}
\end{table}

\subsection{Hyperparameter Selection and Robustness}
We conduct a sensitivity analysis on the two regularization coefficients in the Diverse Pool Criteria: $\lambda_{\text{freq}}$ and $\lambda_{\text{orth}}$. As shown in Figures~\ref{freq} and~\ref{orth}, we vary one hyperparameter while fixing the other to examine their individual influence on model generalization.
In Figure~\ref{freq}, we observe that increasing $\lambda_{\text{freq}}$ generally enhances performance until $\lambda_{\text{freq}} = 1.0$, after which accuracy drops. This indicates that moderate frequency regularization encourages a balanced usage of prompt pairs, leading to better generalization. Excessive regularization, however, may suppress informative prompts.
In Figure~\ref{orth}, a similar trend is observed: $\lambda_{\text{orth}} = 1.0$ consistently achieves the highest performance across different $\lambda_{\text{freq}}$ values. This shows that moderate orthogonality encourages semantic diversity among prompt pairs without over-constraining the feature space.
Together, these results suggest that setting both $\lambda_{\text{freq}}$ and $\lambda_{\text{orth}}$ to 1.0 achieves the best trade-off, leading to improved harmonic accuracy in cross-dataset scenarios.

\begin{table}[t]
\caption{\textbf{Effect of Prompt Pool Size.} Performance comparison across different pool sizes $P$. Results are reported on the ``From E4D to EK'' setting.}
\label{tab:pool_size}
\centering
\small
\begin{tabular}{@{}c|ccc|ccc@{}}
\hline
\multirow{2}{*}{Pool Size $P$} & \multicolumn{3}{c|}{Nouns (\%)} & \multicolumn{3}{c}{Verbs (\%)} \\
\cline{2-7}
 & E4D & EK & hm & E4D & EK & hm \\
\hline
4  & 41.60 & 28.58 & 33.88 & \textbf{36.14} & 46.50 & 40.67 \\
8  & 42.32 & \textbf{30.00} & 35.11 & 34.98 & 47.20 & 40.18 \\
\rowcolor{blue!10}
16 & \textbf{42.93} & 29.71 & \textbf{35.12} & 35.75 & \textbf{47.89} & \textbf{40.94} \\
20 & 42.60 & 29.30 & 34.87 & 35.02 & 47.50 & 40.26 \\
24 & 42.43 & 28.92 & 34.56 & 34.60 & 46.80 & 39.85 \\
28 & 42.31 & 28.63 & 34.34 & 34.17 & 46.42 & 39.51 \\
32 & 42.70 & 29.11 & 34.62 & 33.26 & 45.84 & 38.55 \\
\hline
\end{tabular}
\end{table}

\subsection{More Results of Pool Size}
To further investigate the impact of the prompt pool size $P$, we extend our analysis by incorporating intermediate sizes ($P = 20, 24, 28$) in addition to the original settings ($P = 4, 8, 16, 32$). As shown in Table~\ref{tab:pool_size}, the generalization performance—especially on the unseen EK dataset—improves as $P$ increases from 4 to 16. This improvement is attributed to the growing diversity and expressive capacity of the prompt pool, which helps capture more representative latent interaction patterns across components.

The optimal performance is observed at $P = 16$, achieving the highest harmonic mean accuracy on both nouns (35.12\%) and verbs (40.94\%). Beyond this point, however, performance begins to degrade. For instance, increasing $P$ to 28 leads to a drop of 0.78\% (noun hm) and 1.43\% (verb hm) compared to the peak performance at $P = 16$. This indicates that excessively large prompt pools may introduce semantic redundancy, reducing the effectiveness of pattern selection and weakening the generalization to new domains.

These results highlight that a moderate prompt pool size (e.g., $P=16$) provides a favorable balance between prompt diversity and selection reliability, ensuring both discriminative capability and efficient interaction modeling.
